# Supplementary material for: VADet: Multi-frame LiDAR 3D Object Detection using Variable Aggregation
Source: arXiv:2411.13186 source file (2024-11-20)
Supplement: Supplementary file 1 [file supp.tex]

\begin{appendix}
\title{Supplementary Materials}
\maketitle

In this supplementary, we present the results for the pedestrian class and the full breakdown of performance by both speed and point cloud density.

\section{Results for Pedestrian}
While the trade-off factors analyzed in the main text, speed and point cloud density, are most noticeable for vehicles and allowed VADet to achieve impressive results in the vehicle category, additional experiments indicate that VADet is also effective for pedestrians. As shown in \cref{tab:results-sota-test-pedestrian}, by directing applying VADet without modification, VADet is able to achieve SOTA performance in the pedestrian category, outperforming all LiDAR-only methods and three recent camera-LiDAR fusion methods.

\section{Full breakdown results}
As in the main text, we divide vehicle speed into stationary ($<$0.2\,m/s), slow ([0.2,10)\,m/s), and fast ($\geq$10\,m/s), and point cloud density into sparse ($<$2\,pts/m$^2$), medium ([2,100)\,pts/m$^2$), and dense ($\geq$100\,pts/m$^2$) subcategories. We consider each speed and point cloud density combination and perform evaluation on all subcategories. \Cref{tab:subset-statistics} shows the composition of vehicles in the Waymo dataset. The results are presented in~\Cref{tab:results-vehicle-full}. 

\newpage
As briefly mentioned in the main text, while we notice a performance trade-off between dynamic objects with different point cloud densities, we do not observe this effect for stationary objects, which is likely due to the stationary object point clouds being inherently well-aligned and coherent after aggregation. Using more frames therefore does not introduce distortions that could deteriorate the detection performance.

\begin{table}[t]
\centering
\caption{Overall Pedestrian performance on the Waymo test split compared with other methods (without TTA or ensemble).}
% The best performance according to APH is highlighted in bold and the second best is underlined.}
\resizebox{0.9\linewidth}{!}{%
\begin{tabular}{l|c|c|c}
\toprule
\textbf{Method} & \textbf{\# frames} & \textbf{Modality} & \textbf{L2 AP/APH} \\ \midrule
AFDetV2 & 2 & L & 75.5/72.4 \\
PV-RCNN++ & 2 & L & 76.6/73.6 \\
SWFormer & 3 & L & 75.9/72.1 \\
PillarNeXt-B & 3 & L & 78.8/76.0 \\
FSD++ & 7 & L & 79.0/76.2 \\
3D-MAN & 16 & L & 64.0/60.3 \\
MPPNet & 16 & L & 78.4/75.9 \\
CenterFormer & 16 & L & 80.1/77.4 \\ \midrule
BEVFusion & 3 & C+L & 79.1/76.4 \\
DeepFusion & 5 & C+L & 79.2/76.4 \\
HorizonLiDAR3D & 5 & C+L & 79.3/76.5  \\
LoGoNet & 5 & C+L & \textbf{81.6/78.9} \\ \midrule
VADet-VoxelNeXt & 3--16 & L & {\ul 80.4/78.1} \\ \bottomrule
\end{tabular}%
}
\label{tab:results-sota-test-pedestrian}
\end{table}

\begin{table*}
\caption{The percentage of Waymo vehicles in each speed-density subcategory.}
\label{tab:subset-statistics}
\resizebox{\textwidth}{!}{%
\begin{tabular}{c|ccc|cccc|cccc|cccc}
\toprule
Speed & \multicolumn{3}{c|}{All} & \multicolumn{4}{c|}{Stationary} & \multicolumn{4}{c|}{Slow} & \multicolumn{4}{c}{Fast} \\ 
Density & Sparse & Med. & Dense & All & Sparse & Med. & Dense & All & Sparse & Med. & Dense & All & Sparse & Med. & Dense \\ \midrule
\% & 33.5 & 59.8 & 6.7 & 79.7 & 28.7 & 46.0 & 5.0 & 14.2 & 3.5 & 9.4 & 1.3 & 6.1 & 1.4 & 4.3 & 0.4 \\ \bottomrule
\end{tabular}%
}
\end{table*}

% As briefly mentioned in the main text, while we notice a performance trade-off between dynamic objects with different point cloud densities, we do not observe this effect for stationary objects. This is illustrated in~\cref{fig:stationary_density_vs_frames}, which plots the stationary vehicle performance given in~\Cref{tab:results-vehicle-full}. This is likely due to the stationary object point clouds being inherently well-aligned and coherent after aggregation. Using more frames therefore does not introduce distortions that could deteriorate the detection performance.

% \begin{figure}[t]
%     \centering
%     \begin{subfigure}[b]{0.325\textwidth}
%          \centering
%          \includegraphics[width=\textwidth]{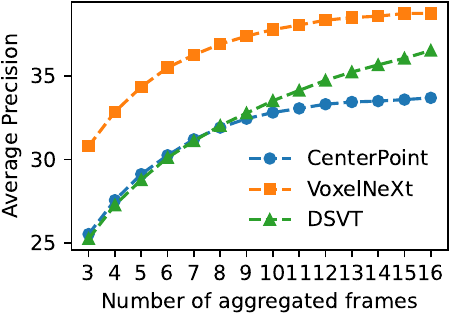}
%          \caption{Sparse}
%          \label{fig:stationary_sparse_vs_frames}
%      \end{subfigure}
%      \hfill
%      \begin{subfigure}[b]{0.325\textwidth}
%          \centering
%          \includegraphics[width=\textwidth]{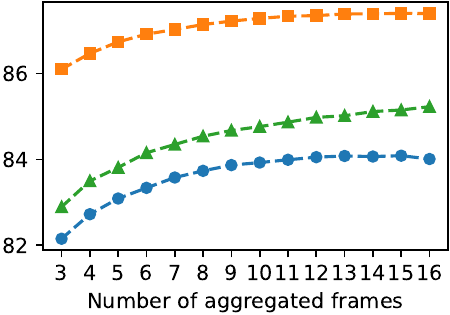}
%          \caption{Medium}
%          \label{fig:stationary_medium_vs_frames}
%      \end{subfigure}
%      \hfill
%      \begin{subfigure}[b]{0.325\textwidth}
%          \centering
%          \includegraphics[width=\textwidth]{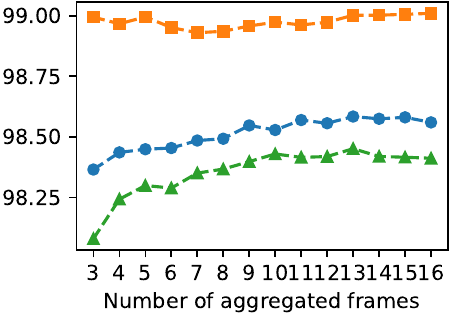}
%          \caption{Dense}
%          \label{fig:stationary_dense_vs_frames}
%      \end{subfigure}
%     \caption{AP vs. the number of frames for stationary vehicles with sparse (<2\,pts/m$^2$), medium ((2,100]\,pts/m$^2$), and dense (>100 pts/m$^2$) point clouds.}
%     \label{fig:stationary_density_vs_frames}
% \end{figure}

\begin{table*}
\caption{AP performance breakdown by speed and point cloud density. The best performance is highlighted in bold.}
\label{tab:results-vehicle-full}
\resizebox{\textwidth}{!}{%
\begin{tabular}{c|c|c|c|cccccccccccccc}
\toprule
\textbf{Architecture} & \textbf{Speed} & \textbf{Density} & \textbf{VADet} & \textbf{3f} & \textbf{4f} & \textbf{5f} & \textbf{6f} & \textbf{7f} & \textbf{8f} & \textbf{9f} & \textbf{10f} & \textbf{11f} & \textbf{12f} & \textbf{13f} & \textbf{14f} & \textbf{15f} & \textbf{16f} \\ \midrule
\multirow{15}{*}{CenterPoint} & \multirow{3}{*}{All} & Sparse & \textbf{35.5} & 25.3 & 27.2 & 28.6 & 29.6 & 30.4 & 31.0 & 31.4 & 31.7 & 31.8 & 32.0 & 32.1 & 32.1 & 32.1 & 32.1 \\
 &  & Medium & \textbf{85.0} & 83.4 & 83.8 & 84.1 & 84.3 & 84.5 & 84.6 & 84.7 & 84.7 & 84.7 & 84.8 & 84.8 & 84.7 & 84.7 & 84.6 \\
 &  & Dense & \textbf{98.7} & 98.5 & 98.5 & 98.5 & 98.6 & 98.6 & 98.6 & 98.6 & 98.6 & 98.6 & 98.6 & 98.6 & 98.6 & 98.6 & 98.5 \\ \cmidrule(l){2-18} 
 & \multirow{4}{*}{Stationary} & All & \textbf{70.3} & 65.8 & 66.8 & 67.6 & 68.1 & 68.5 & 68.8 & 69.1 & 69.3 & 69.4 & 69.5 & 69.6 & 69.6 & 69.7 & 69.7 \\
 &  & Sparse & \textbf{36.8} & 25.5 & 27.6 & 29.1 & 30.2 & 31.2 & 31.9 & 32.4 & 32.8 & 33.1 & 33.3 & 33.4 & 33.5 & 33.6 & 33.7 \\
 &  & Medium & \textbf{84.2} & 82.2 & 82.7 & 83.1 & 83.3 & 83.6 & 83.7 & 83.9 & 83.9 & 84.0 & 84.1 & 84.1 & 84.1 & 84.1 & 84.0 \\
 &  & Dense & \textbf{98.6} & 98.4 & 98.4 & 98.4 & 98.5 & 98.5 & 98.5 & 98.5 & 98.5 & 98.6 & 98.6 & 98.6 & 98.6 & 98.6 & 98.6 \\ \cmidrule(l){2-18} 
 & \multirow{4}{*}{Slow} & All & \textbf{75.0} & 74.1 & 74.5 & 74.7 & 74.9 & 74.9 & 74.8 & 74.8 & 74.7 & 74.6 & 74.6 & 74.5 & 74.4 & 74.2 & 74.0 \\
 &  & Sparse & \textbf{25.9} & 22.2 & 23.7 & 24.5 & 25.0 & 25.0 & 25.0 & 25.1 & 24.9 & 24.6 & 24.6 & 24.2 & 24.1 & 23.7 & 23.3 \\
 &  & Medium & \textbf{86.6} & 86.3 & 86.4 & 86.5 & 86.5 & 86.5 & 86.5 & 86.4 & 86.4 & 86.3 & 86.2 & 86.2 & 86.1 & 86.0 & 85.8 \\
 &  & Dense & \textbf{99.2} & 99.2 & 99.2 & 99.2 & 99.2 & 99.2 & 99.1 & 99.1 & 99.0 & 99.0 & 99.0 & 98.9 & 98.8 & 98.7 & 98.7 \\ \cmidrule(l){2-18} 
 & \multirow{4}{*}{Fast} & All & \textbf{79.5} & 78.9 & 79.0 & 79.1 & 79.0 & 78.9 & 78.9 & 78.8 & 78.6 & 78.3 & 77.9 & 77.8 & 77.4 & 77.0 & 76.6 \\
 &  & Sparse & \textbf{32.1} & 29.8 & 30.4 & 30.8 & 30.6 & 30.4 & 30.0 & 29.8 & 29.3 & 28.8 & 28.2 & 27.8 & 27.0 & 26.4 & 25.4 \\
 &  & Medium & \textbf{90.3} & 90.1 & 90.0 & 90.0 & 89.9 & 89.9 & 89.9 & 89.7 & 89.7 & 89.3 & 89.0 & 89.0 & 88.6 & 88.3 & 88.0 \\
 &  & Dense & 97.8 & 97.8 & 97.8 & 97.7 & 97.8 & 97.7 & 97.8 & 97.8 & \textbf{97.9} & 97.8 & 97.8 & \textbf{97.9} & 97.8 & \textbf{97.9} & 97.8 \\ \midrule
\multirow{15}{*}{VoxelNeXt} & \multirow{3}{*}{All} & Sparse & \textbf{40.1} & 30.6 & 32.5 & 33.9 & 35.0 & 35.7 & 36.2 & 36.6 & 36.9 & 37.1 & 37.3 & 37.4 & 37.4 & 37.5 & 37.4 \\
 &  & Medium & \textbf{88.6} & 87.2 & 87.6 & 87.8 & 87.9 & 88.0 & 88.1 & 88.1 & 88.2 & 88.2 & 88.2 & 88.2 & 88.2 & 88.1 & 88.1 \\
 &  & Dense & 98.9 & \textbf{99.1} & \textbf{99.1} & \textbf{99.1} & \textbf{99.1} & 99.0 & 99.0 & 99.0 & \textbf{99.1} & 99.0 & 99.0 & \textbf{99.1} & \textbf{99.1} & \textbf{99.1} & \textbf{99.1} \\ \cmidrule(l){2-18} 
 & \multirow{4}{*}{Stationary} & All & \textbf{74.3} & 70.4 & 71.3 & 71.9 & 72.3 & 72.6 & 72.9 & 73.1 & 73.2 & 73.3 & 73.4 & 73.5 & 73.5 & 73.6 & 73.6 \\
 &  & Sparse & \textbf{41.2} & 30.8 & 32.9 & 34.4 & 35.5 & 36.3 & 36.9 & 37.4 & 37.8 & 38.1 & 38.4 & 38.5 & 38.6 & 38.8 & 38.8 \\
 &  & Medium & \textbf{87.7} & 86.1 & 86.5 & 86.7 & 86.9 & 87.0 & 87.1 & 87.2 & 87.3 & 87.3 & 87.4 & 87.4 & 87.4 & 87.4 & 87.4 \\
 &  & Dense & 98.8 & \textbf{99.0} & \textbf{99.0} & \textbf{99.0} & \textbf{99.0} & 98.9 & 98.9 & \textbf{99.0} & \textbf{99.0} & \textbf{99.0} & \textbf{99.0} & \textbf{99.0} & \textbf{99.0} & \textbf{99.0} & \textbf{99.0} \\ \cmidrule(l){2-18} 
 & \multirow{4}{*}{Slow} & All & \textbf{79.6} & 78.5 & 78.9 & 79.2 & 79.3 & 79.4 & 79.4 & 79.3 & 79.3 & 79.2 & 79.2 & 79.1 & 78.9 & 78.8 & 78.7 \\
 &  & Sparse & \textbf{30.8} & 27.3 & 28.5 & 29.6 & 30.1 & 30.4 & 30.3 & 30.4 & 30.2 & 29.9 & 29.7 & 29.5 & 29.1 & 28.8 & 28.5 \\
 &  & Medium & \textbf{90.4} & 89.9 & 90.1 & 90.2 & 90.2 & 90.2 & 90.2 & 90.1 & 90.1 & 90.1 & 90.0 & 90.0 & 89.9 & 89.8 & 89.7 \\
 &  & Dense & \textbf{99.6} & \textbf{99.6} & \textbf{99.6} & \textbf{99.6} & \textbf{99.6} & \textbf{99.6} & 99.5 & 99.5 & 99.5 & 99.5 & 99.4 & 99.4 & 99.4 & 99.5 & 99.4 \\ \cmidrule(l){2-18} 
 & \multirow{4}{*}{Fast} & All & \textbf{84.2} & 83.6 & 83.8 & 83.8 & 83.9 & 83.8 & 83.7 & 83.6 & 83.5 & 83.3 & 83.2 & 83.0 & 82.6 & 82.4 & 81.9 \\
 &  & Sparse & \textbf{37.8} & 35.9 & 36.4 & 36.5 & 36.8 & 36.7 & 36.3 & 35.7 & 35.1 & 34.5 & 34.3 & 33.8 & 32.7 & 32.4 & 31.3 \\
 &  & Medium & \textbf{93.8} & 93.4 & 93.5 & 93.5 & 93.5 & 93.4 & 93.4 & 93.4 & 93.3 & 93.2 & 93.1 & 93.0 & 92.7 & 92.5 & 92.2 \\
 &  & Dense & 98.3 & \textbf{98.8} & 98.7 & 98.6 & 98.7 & 98.6 & 98.6 & 98.6 & 98.6 & 98.7 & \textbf{98.8} & 98.7 & 98.7 & \textbf{98.8} & 98.6 \\ \midrule
\multirow{15}{*}{DSVT-P} & \multirow{3}{*}{All} & Sparse & \textbf{36.8} & 25.2 & 27.0 & 28.4 & 29.5 & 30.4 & 31.2 & 31.9 & 32.5 & 33.1 & 33.6 & 34.0 & 34.4 & 34.7 & 35.1 \\
 &  & Medium & \textbf{87.2} & 84.1 & 84.6 & 84.8 & 85.1 & 85.2 & 85.3 & 85.4 & 85.5 & 85.6 & 85.6 & 85.6 & 85.7 & 85.7 & 85.8 \\
 &  & Dense & \textbf{98.8} & 98.3 & 98.4 & 98.4 & 98.4 & 98.4 & 98.4 & 98.4 & 98.4 & 98.4 & 98.4 & 98.4 & 98.4 & 98.3 & 98.3 \\ \cmidrule(l){2-18} 
 & \multirow{4}{*}{Stationary} & All & \textbf{72.3} & 66.4 & 67.4 & 68.1 & 68.7 & 69.1 & 69.5 & 69.8 & 70.1 & 70.3 & 70.6 & 70.7 & 70.9 & 71.0 & 71.2 \\
 &  & Sparse & \textbf{38.1} & 25.2 & 27.3 & 28.8 & 30.1 & 31.1 & 32.0 & 32.8 & 33.5 & 34.1 & 34.7 & 35.2 & 35.7 & 36.1 & 36.5 \\
 &  & Medium & \textbf{86.4} & 82.9 & 83.5 & 83.8 & 84.2 & 84.3 & 84.5 & 84.7 & 84.8 & 84.9 & 85.0 & 85.0 & 85.1 & 85.2 & 85.2 \\
 &  & Dense & \textbf{98.8} & 98.1 & 98.2 & 98.3 & 98.3 & 98.4 & 98.4 & 98.4 & 98.4 & 98.4 & 98.4 & 98.5 & 98.4 & 98.4 & 98.4 \\ \cmidrule(l){2-18} 
 & \multirow{4}{*}{Slow} & All & \textbf{77.3} & 75.0 & 75.4 & 75.5 & 75.6 & 75.7 & 75.6 & 75.5 & 75.5 & 75.5 & 75.5 & 75.5 & 75.4 & 75.3 & 75.3 \\
 &  & Sparse & \textbf{25.9} & 22.4 & 23.4 & 23.9 & 24.2 & 24.3 & 24.4 & 24.5 & 24.6 & 24.6 & 24.7 & 24.7 & 24.7 & 24.6 & 24.7 \\
 &  & Medium & \textbf{88.5} & 86.5 & 86.7 & 86.7 & 86.7 & 86.7 & 86.6 & 86.5 & 86.5 & 86.5 & 86.4 & 86.3 & 86.3 & 86.3 & 86.2 \\
 &  & Dense & \textbf{99.5} & 99.2 & 99.2 & 99.2 & 99.2 & 99.2 & 98.9 & 98.9 & 98.8 & 98.8 & 98.7 & 98.7 & 98.5 & 98.4 & 98.5 \\ \cmidrule(l){2-18} 
 & \multirow{4}{*}{Fast} & All & \textbf{82.6} & 81.2 & 81.2 & 81.0 & 80.9 & 80.8 & 80.7 & 80.7 & 80.6 & 80.6 & 80.5 & 80.5 & 80.4 & 80.3 & 80.2 \\
 &  & Sparse & \textbf{33.1} & 30.7 & 31.2 & 31.2 & 31.1 & 31.1 & 30.9 & 30.9 & 30.8 & 30.7 & 30.5 & 30.4 & 30.2 & 29.9 & 29.5 \\
 &  & Medium & \textbf{92.9} & 91.6 & 91.5 & 91.4 & 91.3 & 91.1 & 91.0 & 90.9 & 90.9 & 90.8 & 90.8 & 90.9 & 90.7 & 90.6 & 90.6 \\
 &  & Dense & 97.5 & \textbf{97.6} & 97.2 & 97.2 & 97.1 & 96.8 & 97.0 & 96.9 & 96.8 & 96.7 & 96.9 & 97.0 & 96.8 & 96.8 & 96.7 \\ \bottomrule
\end{tabular}%
}
\end{table*}

\end{appendix}
